# Supplementary material for: Orthogonal Inference for Conditional Z-Estimation without Cross-Fitting: A Distributional Nearest-Neighbor Approach
Source: arXiv:2610.38965 source file (2026-10-28)
Supplement: Supplementary file 1 [file affine_supplement_layout.tex]

% Supplement-only display layout; body typography remains with elsarticle.
\input{affine_layout.tex}

\ifpreprint
  \renewcommand{\arraystretch}{1.0}
\else
  \renewcommand{\arraystretch}{1.12}
\fi
\setlength{\abovecaptionskip}{5pt}
\setlength{\belowcaptionskip}{5pt}
\setlength{\intextsep}{14pt plus 2pt minus 2pt}
